# Supplementary material for: Semantic Graphs for Syntactic Simplification: A Revisit from the Age of LLM
Source: arXiv:2407.04067 source file (2024-07-04)
Supplement: Supplementary file 1 [file appendix.tex]

\appendix
\section{Prompts}
\label{sec:appendix}

\vspace{1ex}
\begin{prompt}[title={Prompt \thetcbcounter: AMR Subgraph Prompting}, label=prompt:sub-amr]
    \texttt{[User]} \texttt{[...]} The AMR is split into subgraphs where each subgraph roots at a predicate. \\
    \# Paragraph\\
    \texttt{\{complex sentence\}}\\
    \# AMR Subgraphs\\
    \#\# Subgraph 1 \\
    \texttt{\{amr-1\}} \texttt{[...]}

\end{prompt}
